# Supplementary material for: Efficient State Space Model via Fast Tensor Convolution and Block Diagonalization
Source: arXiv:2402.15290 source file (2025-05-05)
Supplement: Supplementary file 1 [file 8-appendix.tex]

\appendix
\section*{Appendix}
Our appendix provides detailed information on the experimental setup, dataset, code implementation, etc. The full appendix can be found on arXiv: \href{https://arxiv.org/abs/2402.15290}{https://arxiv.org/abs/2402.15290}.
